# Supplementary material for: Interactive Optimization of Generative Image Modeling using Sequential Subspace Search and Content-based Guidance
Source: arXiv:1906.09840 source file (2020-08-29)
Supplement: Supplementary file 1 [file supp-crowdsource.tex]

\section{Crowdsourced Evaluation Details}
\label{sec:supp_crowd}
We conducted the crowdsourced evaluation using Amazon Mechanical Turk.
Specifically, we showed the reference image on top identified as ``A'' and the two edited images on the bottom identified as ``B'' and ``C''. 
We then asked: ``Which of the two images on the bottom ``B'' or ``C'' better matches image ``A''? 
The answer options were ``B'', ``C''. 
We randomly shuffle the edited result using our method and result to be ``B'' and ``C'' for each query.
The described interface is shown in \figname~\ref{fig:amt_ui}.
And we show the detail voting results in \figname~\ref{fig:amt_result_separate}.

\begin{figure}
    \centering
    \includegraphics[width=\linewidth]{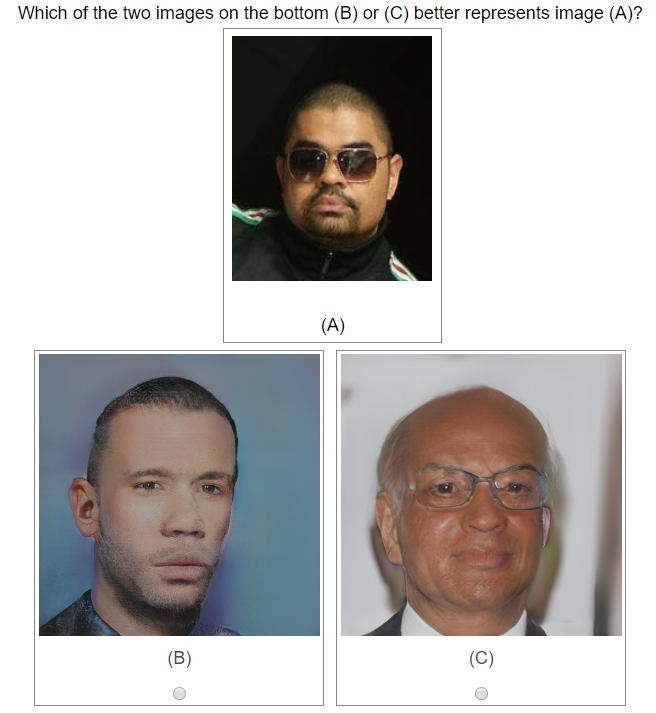}
    \caption{The user interface of our comparison user study conducted on Amazon Mechanical Turk.}
    \label{fig:amt_ui}
\end{figure}

\begin{figure}
\centering
\includegraphics[width=\linewidth]{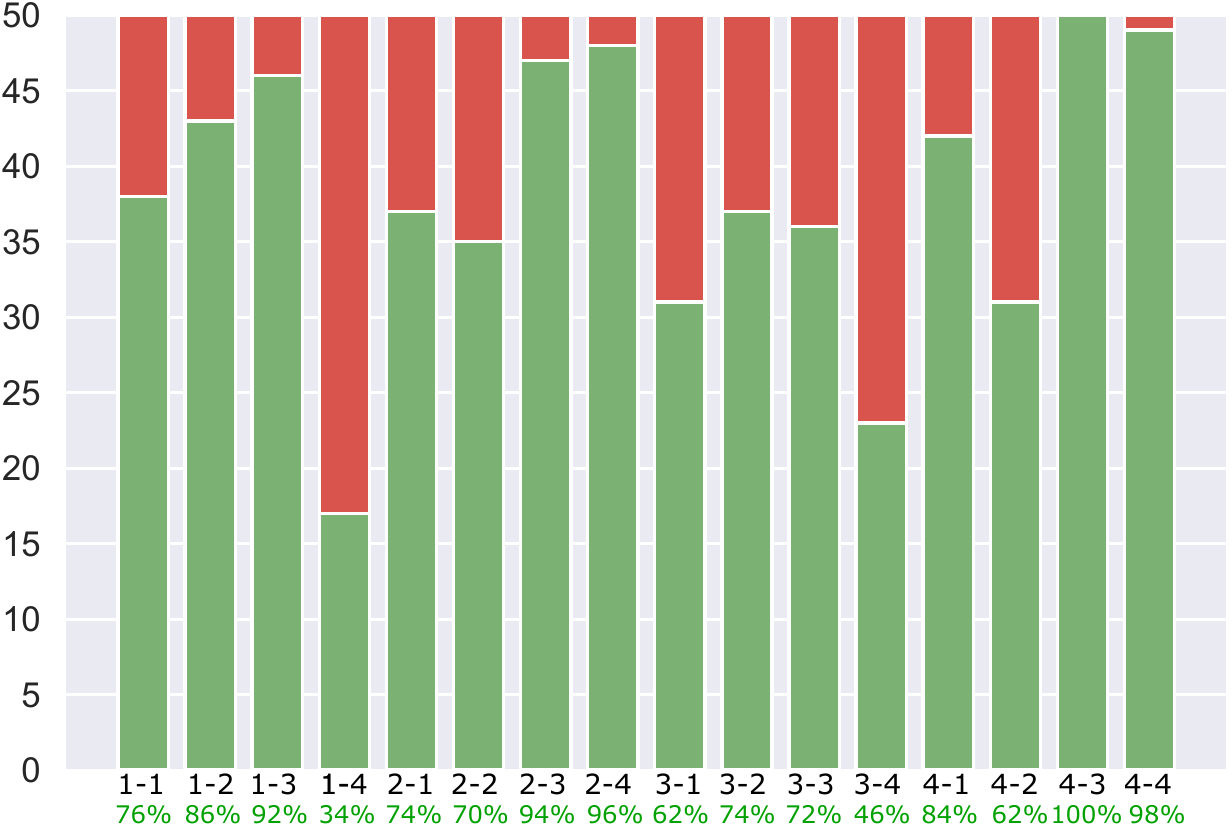}
\caption{
The detail voting results from crowdworkers, the green bar denotes the vote for our method, and the red bar denotes the vote for iGAN.
For each question, there are total 50 votes.
The green number indicates the vote percentage of our method.
Please find the corresponding images in \figname 11 in the main paper and the rest of the result images in the detail result supplemental material (1-1 indicates the 1st result of reference image 1).
% \figname~\ref{fig:supp_us_result}  
}
\label{fig:amt_result_separate}
\end{figure}
