# Supplementary material for: Interactive Optimization of Generative Image Modeling using Sequential Subspace Search and Content-based Guidance
Source: arXiv:1906.09840 source file (2020-08-29)
Supplement: Supplementary file 2 [file supp-intro.tex]

\section{Introduction}
In this supplemental material we include the following items that further highlight the effectiveness of our system and assist the reader to understand this work.

\paragraph{Additional User studies (\secname~\ref{sec:supp_us})} 
We conducted an additional user studies: \textit{synthetic target study} (\secname~\ref{syn-target-study}) to provides another quantitative comparison between our method and \mbox{iGAN~\cite{iGAN2016}}. 
% \paragraph{Result details using our framework (\secname~\ref{addit-result})} 
% \hl{
% In the main paper we demonstrate our method can be plug-and-play with different generators (\mbox{\eg~MUNIT~\cite{MUNIT}, ProgressiveGAN~\cite{Karras2018ICLR} and AttnGAN~\cite{attngan}}) and only show part of the manipulation sequences.
% Here we include the complete manipulation sequences for all the results shown in the main paper to help the user better understand how our framework provides useful assist for generating desired images.
% % of all three systems to show the versatility of our system.
% }
\paragraph{Interface and voting result of Crowdsourced Evaluation (\secname~\ref{sec:supp_crowd})} 
Here we provide the detail description of the interface we used in the crowdsourced evalution.
Also, we show the complete voting results of crowdworkers.

% \paragraph{High dimensional Bayesian Optimization discussion (\secname~\ref{sec:high_discuss})}
% Here we provide some additional insights and theories to explain why our method performs well on high dimensional latent space.
