# Supplementary material for: Interactive Optimization of Generative Image Modeling using Sequential Subspace Search and Content-based Guidance
Source: arXiv:1906.09840 source file (2020-08-29)
Supplement: Supplementary file 3 [file supp-userstudy.tex]

\section{Additional user study results}

\begin{figure}
    \centering
    \includegraphics[width=\linewidth]{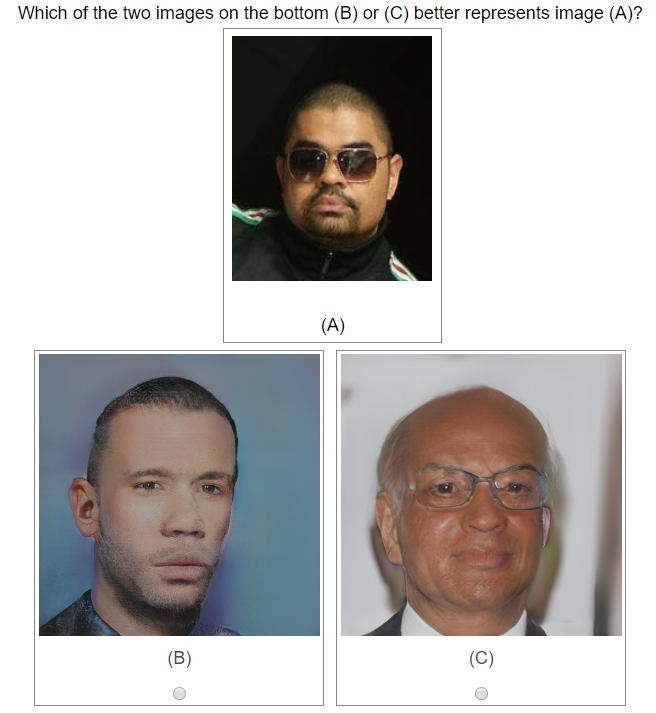}
    \caption{The user interface of our comparison user study conducted on Amazon Mechanical Turk.}
    \label{fig:amt_ui}
\end{figure}

% \begin{figure}
% \centering
% \includegraphics[width=\linewidth]{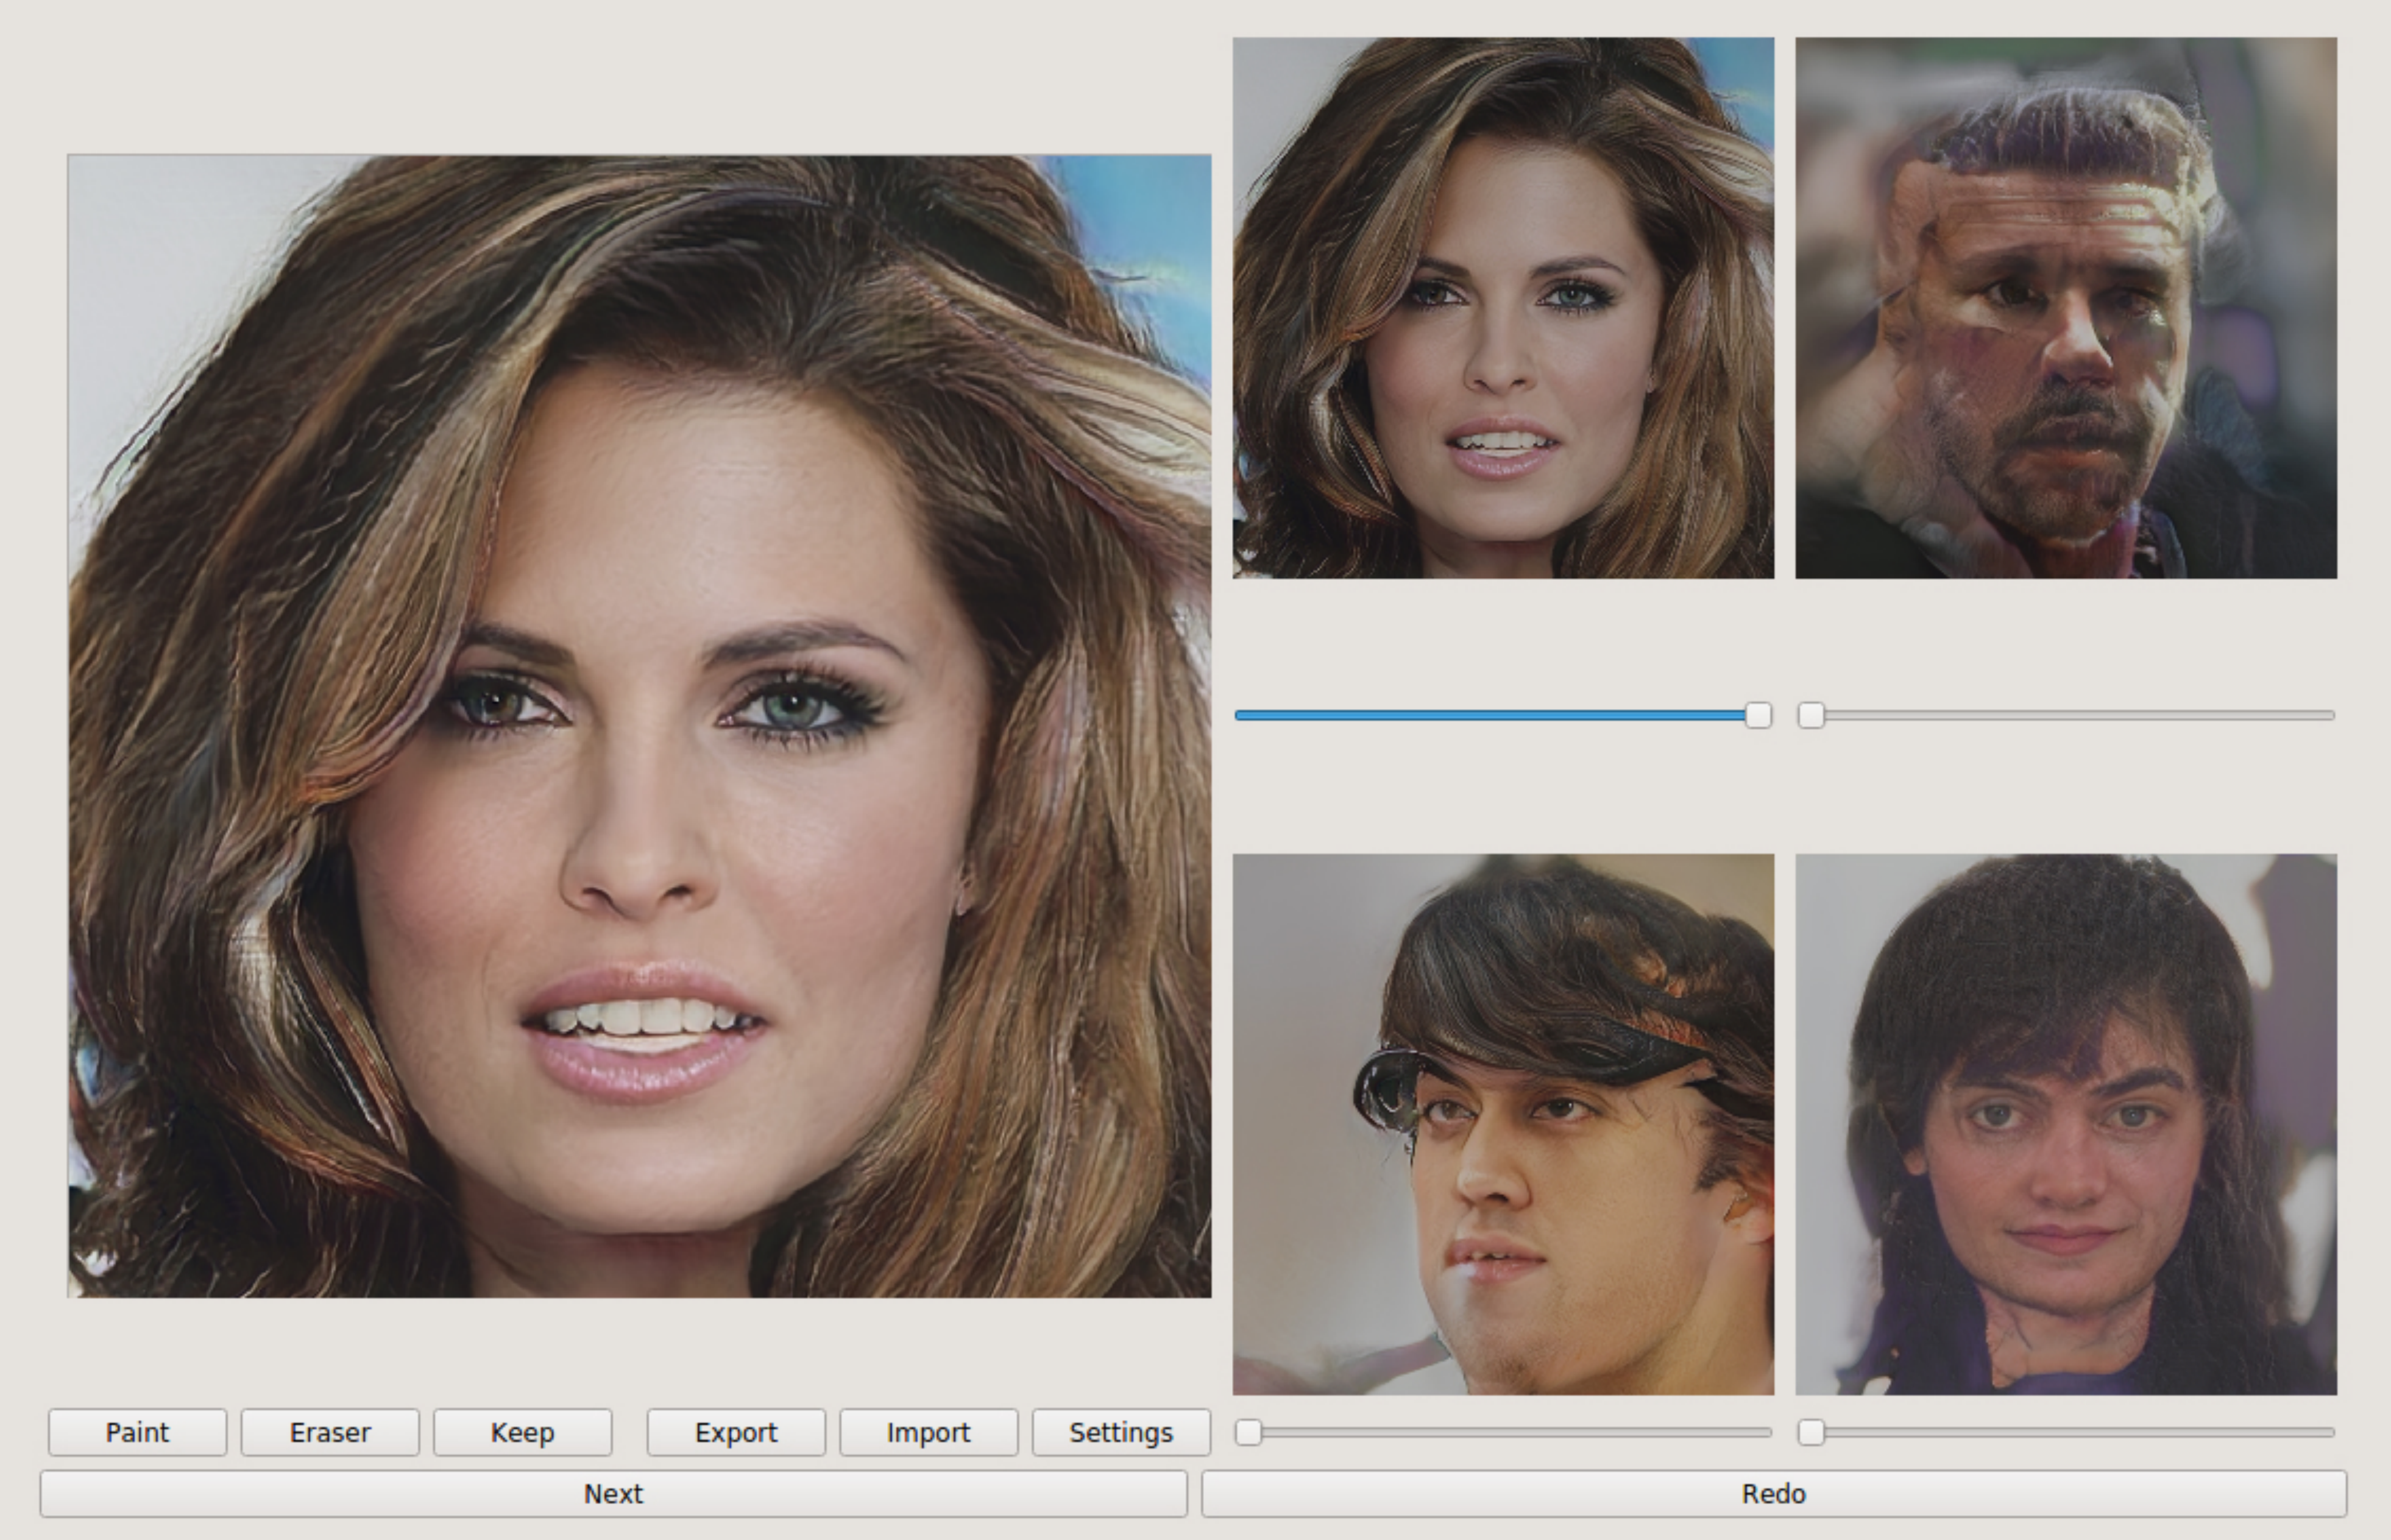}
% \caption{
% Screenshot of our user interface. 
% }
% \label{fig:ui_screenshot}
% \end{figure}

\begin{figure}
\centering
\includegraphics[width=\linewidth]{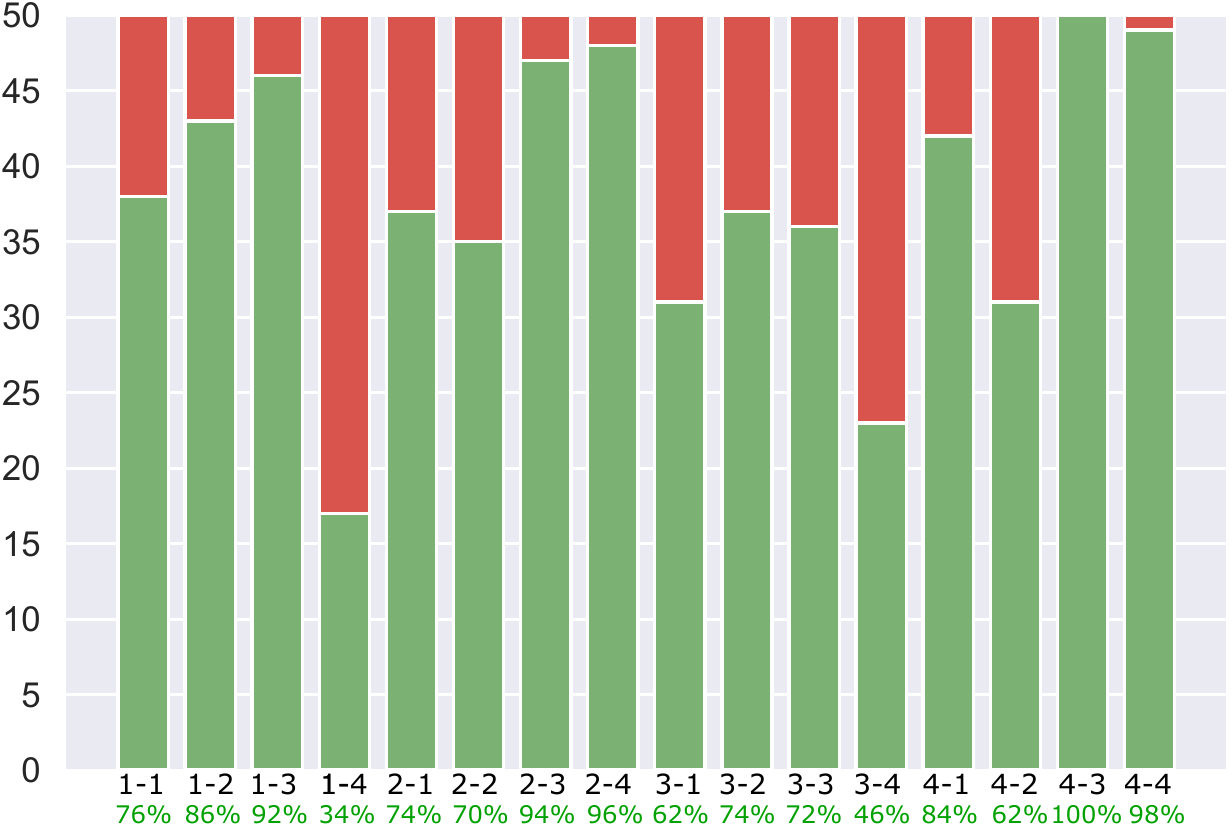}
\caption{
The detail voting results from crowdworkers, the green bar denotes the vote for our method, and the red bar denotes the vote for iGAN.
For each question, there are total 50 votes.
The green number indicates the vote percentage of our method.
Please find the corresponding images in \figname 11 in the main paper and the rest of the result images in the detail result supplemental material (1-1 indicates the 1st result of reference image 1).
% \figname~\ref{fig:supp_us_result}  
}
\label{fig:amt_result_separate}
\end{figure}

% \subsection{Discussion}
% In this section we discuss possible reason why our system outperforms iGAN. We discuss two main potential reasons, user incapability of expressing their preference in drawing and out-of-distribution input, that leads to better match of user preference in our system compares to iGAN. 
% \paragraph{User incapability of expressing their preference}
% iGAN demonstrated their method with drawing of outdoor terrain, which is rather easy to draw compare to our user study. They did not account for the fact that 
